# Supplementary material for: Revisiting Kernel Attention with Correlated Gaussian Process Representation
Source: arXiv:2502.20525 source file (2025-02-27)
Supplement: Supplementary file 1 [file old_appendix.tex]

% \subsection{Variational inference...}
%     \textbf{Variational inference}. To do variational inference, let us define $m \leq n$ auxiliary variables $\textbf{u} \in \mathbb{R}^m$ where $u_i = s(k_i)$. We can view the keys $(\textbf{k}_1,\ldots, \textbf{k}_m)$ as the inducing points in variational inference of the standardized GP model (\ref{eq: standardized GP model}). The distribution of $\textbf{u}$ is Gaussian:
%     \begin{align*}
%         p(\textbf{u}) = \mathcal{N}(\textbf{0}, \textbf{K}_{\textbf{uu}}),
%     \end{align*}
%     where $[\textbf{K}_{\textbf{uu}}]_{ij}= k_s(\textbf{k}_i, \textbf{k}_j)$.
%     The cross-covariance between input $\textbf{x}_i$ and inducing key $\textbf{k}_j$ is calculated as:
%     \begin{align}
%         k_{f_Q,u} (\textbf{x}_i, \textbf{k}_j) &= E[\sigma_{f_Q}s(\textbf{x}_i\textbf{W}_Q^T)s(\textbf{k}_j)] \\
%         &= E[\sigma_{f_Q}s(\textbf{x}_i\textbf{W}_Q^T)s(\textbf{x}_j\textbf{W}_K^T)]\\
%         &=\sigma_{f_Q}exp \Big( \frac{-1}{2} ||\textbf{x}_i\textbf{W}_Q^T-\textbf{x}_j\textbf{W}_K^T ||^2 \Big)=\sigma_{f_Q} k_s(\textbf{q}_i, \textbf{k}_j),
%     \end{align}
%     where $i \in \{1,\ldots,n\}$ and $j \in \{1,\ldots,m \}$. Using this cross-covariance function, we can compute the covariance matrix $\textbf{K}_{\textbf{f}_Q, \textbf{u}} \in \mathbb{R}^{n\times m}$.
%     \par \textcolor{blue}{Long: Can we use variational inference to learn the inducing keys?} 
%     \par The conditional Gaussian distribution is given by:
%     \begin{align}
%         p(\textbf{f}_Q|\textbf{u}) = \mathcal{N}(\textbf{K}_{\textbf{f}_Q, \textbf{u}} \textbf{K}_{\textbf{u}, \textbf{u}}^{-1}\textbf{u}, \textbf{K}_{\textbf{f}_Q, \textbf{f}_Q} + \textbf{K}_{\textbf{f}_Q, \textbf{u}} \textbf{K}_{\textbf{u}, \textbf{u}}^{-1}\textbf{K}_{\textbf{f}_Q, \textbf{u}}^T)
%     \end{align}
%     Consider the mean of $p(\textbf{f}_Q|\textbf{u})$, $\textbf{m} = \textbf{K}_{\textbf{f}_Q, \textbf{u}} \textbf{K}_{\textbf{u}, \textbf{u}}^{-1}\textbf{u} $, if we set the values vector $\textbf{v}:=\textbf{K}_{\textbf{f}_Q, \textbf{u}} \textbf{K}_{\textbf{u}, \textbf{u}}^{-1}\textbf{u}$, we obtain the kernel attention with assymetric kernel $\textbf{K}_{\textbf{f}_Q, \textbf{u}}$.

\textbf{List of works:}
\begin{itemize}
    \item Text:
    \begin{enumerate}
        \item Add one section for characterizing the algorithmic uncertainty calibration (Done)
        \item Edit the experiment details section (In progress)
        \item Insert reproducibility checklist (AISTATS 2024)
    \end{enumerate}
    
    \item Experiments:
    \begin{enumerate}
        \item Improve the results on CIFAR10, CIFAR10C and OOD detection in the main paper and running ablation results
        \item Running experiments for CIFAR100 and CIFAR100C (If have enough time)
    \end{enumerate}
\end{itemize}

\section{Derivation and Practical Implementation of Loss Function}
\label{app:A}
    \textcolor{red}{
        This section further derives a more specific expression for our main objective function in Eq.~\eqref{eq:main_obj}, which is quoted below
        \begin{eqnarray} \label{eq:maximize}
        \max_\theta \Big\{ \mathfrak{L}(\theta) &\triangleq& \log p(\mathbf{z}_a) \ +\ \log p\left(\boldsymbol{\nu}_a \mid \mathbf{z}_a\right) \ - \  \alpha \cdot \mathrm{loss}(\boldsymbol{\nu}_a)\Big\} \ .
        \end{eqnarray}
        where $\boldsymbol{\nu}_a$ and $\mathbf{z}_a$ is defined previously in Eq.~\eqref{eq:cgp_attention}. Here, note that $\boldsymbol{\nu}_a$ is set to be the mean of the predictive Gaussian whose parameters are previously specified in Eq.~\eqref{eq:log Gaussian},
        \begin{eqnarray} 
        p(\boldsymbol{\nu} \mid \mathbf{z}_a) &=& \mathbb{N}\Bigg(\boldsymbol{\nu} \mid \mathcal{K}_{qk}\Big(\mathcal{K}_k + \sigma^2\mathbf{I}\Big)^{-1}\mathbf{z}_a, \mathcal{K}_q - \mathcal{K}_{qk}\Big(\mathcal{K}_k + \sigma^2\mathbf{I}\Big)^{-1}\mathcal{K}_{kq}\Bigg) \nonumber\\
        &=& \mathbb{N}\Bigg(\boldsymbol{\nu} \mid\boldsymbol{\nu}_a, \mathcal{K}_q - \mathcal{K}_{qk}\Big(\mathcal{K}_k + \sigma^2\mathbf{I}\Big)^{-1}\mathcal{K}_{kq}\Bigg)
        \end{eqnarray}
        Thus, let $\boldsymbol{\Sigma} \triangleq \mathcal{K}_q - \mathcal{K}_{qk}\Big(\mathcal{K}_k + \sigma^2\mathbf{I}\Big)^{-1}\mathcal{K}_{kq}$ which characterizes the attention output uncertainty, 
        \begin{eqnarray}
        \log p(\boldsymbol{\nu}_a \mid \mathbf{z}_a) &=& -\ \frac{1}{2}n\log(2\pi) \ -\  \frac{1}{2}\log \left|\mathbf{det}(\boldsymbol{\Sigma})\right|
        \end{eqnarray}
        Thus, plugging the above into the expression of $\mathfrak{L}(\theta)$ along with the fact that $\log\mathbb{N}(\mathbf{z}_a \mid \mathbf{0}, \mathcal{K}_k) = (-n/2)\log(2\pi) - (1/2)\log|\mathbf{det}(\mathcal{K}_k)| - (1/2)\mathbf{z}^\top_a\mathcal{K}_k^{-1}\mathbf{z}_a$, we have
        \begin{eqnarray}
        \hspace{-8mm}\mathfrak{L}(\theta) 
        \hspace{-2mm}&=&\hspace{-2mm} -\  \frac{1}{2} \log |\mathbf{det}(\mathcal{K}_k)| \ - \ \frac{1}{2} \mathbf{z}_a^\top \mathcal{K}_k^{-1} \mathbf{z}_a \ -\ \frac{1}{2} \log |\mathbf{det}(\boldsymbol{\Sigma})| -\ n\log(2\pi) -\ \alpha\cdot\mathrm{loss}(\boldsymbol{\nu}_a)
        \end{eqnarray}
        Maximizing $\mathfrak{L}(\theta)$ is thus equivalent to solving for 
        \begin{eqnarray}
        \hspace{-10.5mm}\theta_\ast &\triangleq&  \min_\theta \Bigg\{\mathfrak{L}'(\theta) \ \triangleq\  \log |\mathbf{det}(\mathcal{K}_k)| \ +\ \mathbf{z}_a^\top \mathcal{K}_k^{-1} \mathbf{z}_a \ +\  \log |\mathbf{det} (\boldsymbol{\Sigma})| \ +\ \alpha \cdot \mathrm{loss}(\boldsymbol{\nu}_a)\Bigg\}
        \end{eqnarray}
        which specifies a parameterization $\theta_\ast$ for the CGP-based attention that balances between (1) minimizing the output uncertainty, which is characterized by the first $3$ terms; and (2) minimizing the transformer's prediction loss, which is characterized by the last term.\\
         Practical Implementation. In practice, we find that the above can be further relaxed to increase the flexibility in balancing between minimizing attention uncertainty and prediction loss via augmenting the above minimization task with an additional parameterized surrogate $\boldsymbol{\nu}(\mathbf{x}; \gamma)$ of the CGP-based attention output, which leads to improved overall performance. This process is detailed below
        \begin{eqnarray}
        \theta_\ast, \gamma_\ast \ \ =\ \  \min_{\theta,\gamma}\ \widehat{\mathfrak{L}}(\theta, \gamma) 
        \end{eqnarray}
        where the augmented minimization loss is defined as
        \begin{eqnarray} 
        \widehat{\mathfrak{L}}(\theta, \gamma) &\triangleq& \Big(\boldsymbol{\nu}(\mathbf{x}; \gamma) - \boldsymbol{\nu}_a\Big)^\top\mathbf{\Sigma}^{-1}\Big(\boldsymbol{\nu}(\mathbf{x}; \gamma) - \boldsymbol{\nu}_a\Big) \ +\ \alpha \cdot \mathrm{loss}(\boldsymbol{\nu}(\mathbf{x}; \gamma))\nonumber\vspace{4mm}\\
        &+& \log \Big|\mathbf{det}(\mathcal{K}_k)\Big| \ +\  \log \Big|\mathbf{det} (\boldsymbol{\Sigma})\Big| \ +\  \mathbf{z}_a^\top \mathcal{K}_k^{-1} \mathbf{z}_a 
        \end{eqnarray}
        This is in fact equivalent to 
        \begin{eqnarray} \label{eq:maximize_augmented}
        \max_{\theta,\gamma} \Big\{ \log p(\mathbf{z}_a) \ +\ \log p\left(\boldsymbol{\nu}(\mathbf{x};\gamma) \mid \mathbf{z}_a\right) \ - \  \alpha \cdot \mathrm{loss}(\boldsymbol{\nu}(\mathbf{x};\gamma))\Big\} \ .
        \end{eqnarray}
        which reduces to the original maximization task in Eq.~\eqref{eq:maximize} when $\gamma$ is selected such that $\boldsymbol{\nu}_a = \boldsymbol{\nu}(\mathbf{x};\gamma)$. Otherwise, if we optimize for $\gamma$ along with $\theta$, it will provide a better handle to balance between minimizing attention uncertainty and prediction loss (as verified empirically).
    }

    \textcolor{blue}{
        This section further derives a more specific expression for our main objective function in Eq.~\eqref{eq:main_obj}, which is quoted below
        \begin{eqnarray} \label{eq:maximize}
        \max_\theta \Big\{ \mathfrak{L}(\theta) &\triangleq& \log E[p(\boldsymbol{\nu}_a|\mathbf{z}_0)] + \log E[p(\mathbf{z}_a|\mathbf{z}_0)] - \  \frac{\alpha}{2} \cdot \mathrm{loss}(\boldsymbol{\nu}_a)\Big\}  \ .
        \end{eqnarray}
        where $\boldsymbol{\nu}_a$ and $\mathbf{z}_a$ is defined previously in Eq.~\eqref{eq:cgp_attention}. Here, note that $\boldsymbol{\nu}_a$ is set to be the mean of the predictive Gaussian whose parameters are previously specified in Eq.~\eqref{eq:log Gaussian}.\\
        Instead of maximizing $\log E[p(\boldsymbol{\nu}_a|\mathbf{z}_0))]$ and $\log E[p(\mathbf{z}_a|\mathbf{z}_0)]$, we optimize their lower bounds as follow.
        According to Jensen's inequality and 
        \begin{align*}
            \boldsymbol{\nu}_a|\mathbf{z}_0 &\sim \mathcal{N}(\mathbf{m}_{q0}, \boldsymbol{\Sigma}_{q0}) \\ 
            &:=  \mathcal{N}(\mathcal{K}_{q0}(\mathcal{K}_0+\sigma^2 \mathbf{I})^{-1}\mathbf{z}_0, \ \mathcal{K}_q-\mathcal{K}_{q0}(\mathcal{K}_0+\sigma I)^{-1}\mathcal{K}_{0q}),
        \end{align*}
        we have
        \begin{equation}
            \begin{aligned}
            \log E[p(\boldsymbol{\nu}_a|\mathbf{z}_0)] &\geq E[\log p(\boldsymbol{\nu}_a|\mathbf{z}_0)] \\
            &= 0.5 \cdot E_{\mathbf{z}_0}[-(\boldsymbol{\nu}_a-\mathbf{m}_{q0})^\top \boldsymbol{\Sigma}_{q0}^{-1}(\boldsymbol{\nu}_a-\mathbf{m}_{q0}) - \log \text{det}(\boldsymbol{\Sigma}_{q0})-n\log 2\pi]\\
            &= -0.5\cdot\int_{\mathbf{z}_0} p(\mathbf{z}_0)[(\boldsymbol{\nu}_a-\mathbf{m}_{q0})^\top \boldsymbol{\Sigma}_{q0}^{-1}(\boldsymbol{\nu}_a-\mathbf{m}_{q0}) + \log \text{det}(\boldsymbol{\Sigma}_{q0})+n\log 2\pi]d\mathbf{z}_0\\
            &= -0.5\cdot\int_{\mathbf{z}_0} p(z_0)[(\boldsymbol{\nu}_a-\mathbf{m}_{q0})^\top \boldsymbol{\Sigma}_{q0}^{-1}(\boldsymbol{\nu}_a-\mathbf{m}_{q0})]d\mathbf{z}_0 -\frac{\log \text{det}(\boldsymbol{\Sigma}_{q0})}{2} - \frac{n\log 2\pi}{2} \\
            &\geq -0.5\cdot \int_{\mathbf{z}_0} p(\mathbf{z}_0)[(\boldsymbol{\nu}_a-\mathbf{m}_{q0})^\top \boldsymbol{\Sigma}_{q0}^{-1}(\boldsymbol{\nu}_a-\mathbf{m}_{q0})]d\mathbf{z}_0  -\frac{|\log \text{det}(\boldsymbol{\Sigma}_{q0})|}{2} - \frac{n\log 2\pi}{2}
            \\
            &\approx -0.5\cdot \frac{1}{n}\sum_{i=1}^n [(\boldsymbol{\nu}_a-\mathbf{m}_{q0}(\mathbf{z}_0^i))^\top \boldsymbol{\Sigma}_{q0}^{-1}(\boldsymbol{\nu}_a-\mathbf{m}_{q0}(\mathbf{z}_0^i))]  -\frac{|\log \text{det}(\boldsymbol{\Sigma}_{q0})|}{2} - \frac{n\log 2\pi}{2},
        \end{aligned}
        \end{equation}  
        where we use Monte-Carlo method to approximate the final integral with  $\mathbf{z}_0^i \sim p(\mathbf{z}_0)=\mathcal{N}(\mathbf{0}, \mathcal{K}_0).$. Using similar argument, we can lower bound $\log E[p(\mathbf{z}_a|\mathbf{z}_0)]$:
        \begin{align}
            \log E[p(\mathbf{z}_a|\mathbf{z}_0)] \geq -0.5\cdot \frac{1}{n}\sum_{i=1}^n [(\mathbf{z}_a-\mathbf{m}_{k0}(\mathbf{z}_0^i))^\top \boldsymbol{\Sigma}_{k0}^{-1}(\mathbf{z}_a-\mathbf{m}_{k0}(\mathbf{z}_0^i))]  -\frac{|\log \text{det}(\boldsymbol{\Sigma}_{k0})|}{2} - \frac{n\log 2\pi}{2}
        \end{align}
        Therefore, our optimization objective becomes
        \begin{equation} \label{eq:maximize full}
            \begin{aligned}
                    \max_\theta \Big\{ \hat{\mathfrak{L}}(\theta) &\triangleq  
                -\frac{1}{n}\sum_{i=1}^n [(\boldsymbol{\nu}_a-\mathbf{m}_{q0}(\mathbf{z}_0^i))^\top \boldsymbol{\Sigma}_{q0}^{-1}(\boldsymbol{\nu}_a-\mathbf{m}_{q0}(\mathbf{z}_0^i))]  -|\log \text{det}(\boldsymbol{\Sigma}_{q0})|\\
                - \frac{1}{n}&\sum_{i=1}^n [(\boldsymbol{z}_a-\mathbf{m}_{k0}(\mathbf{z}_0^i))^\top \boldsymbol{\Sigma}_{k0}^{-1}(\boldsymbol{z}_a-\mathbf{m}_{k0}(\mathbf{z}_0^i))]  -|\log \text{det}(\boldsymbol{\Sigma}_{k0})| - \alpha \cdot \text{loss}(\boldsymbol{\nu}_a) \Big\}
            \end{aligned}
        \end{equation}
    }
    
    \iffalse
    Thus, our original maximization task in \eqref{eq:maximize} can be cast into the following minimization problem
    \begin{equation}
        \begin{aligned}
            \min_\theta \Big\{ \mathfrak{L}'(\theta) \ \ &\triangleq \ \ \log |\mathbf{det}(\mathcal{K}_k)| \ + \ \log |\mathbf{det}(\boldsymbol{\Sigma})| \ +\ \mathbf{z}_a^\top \mathcal{K}_k^{-1} \mathbf{z}_a \\ \ \ &+ \ \ (\boldsymbol{\nu} \ - \ \boldsymbol{\nu}_a)^\top \boldsymbol{\Sigma}^{-1} (\boldsymbol{\nu} \ - \ \boldsymbol{\nu}_a) \ + \  2\alpha \cdot \mathrm{loss}(\boldsymbol{\nu}_a) \Big\}
        \end{aligned}\label{eq:minimize}
    \end{equation}
    \fi
    
    %if the family of surrogate parameters $\gamma$ is sufficiently expressive such that the optimal parameter $\gamma$ that minimizes the prediction loss $\mathrm{loss}(\boldsymbol{\nu}(\mathbf{x};\gamma))$ is also approximately close to the optimal parameter that minimizes the output uncertainty $\boldsymbol{\nu}(\mathbf{x};\gamma) \simeq \boldsymbol{\nu}_a$.

    
    %to increase the flexibility in balancing between fitting a CGP-based attention unit with low uncertainty\footnote{This is achieved via minimizing exclusively the first $2$ terms in Eq.~\eqref{eq:main_obj} or equivalently, the first $4$ terms in Eq.~\eqref{eq:minimize}} and fitting the attention output to minimize the prediction loss, we further parameterize $\boldsymbol{\nu}$ as a learnable function of the queries.
    
        

\section{Analytic form of CGPT's variance}
\textcolor{blue}{
    In Equation \eqref{eq: exp closed form}, we have derived the expectation $\mathbb{E}[\mathbf{z}_q \mid \mathbf{z}_k]$ of the CGP model, which then can be modeled as the predictive mean of CGPT in equation \eqref{eq:cgp_attention}. In order to perform uncertainty calibration, we need to obtain the variance of $\mathbf{z}_q \mid \mathbf{z}_k$. We have the following identity:
    \begin{align} \label{eq: variance formula}
        \mathbb{V}[\mathbf{z}_q \mid \mathbf{z}_k] =  \mathbb{E}[\mathbf{z}_q\mathbf{z}_q^\top\mid \mathbf{z}_k] -  \mathbb{E}[\mathbf{z}_q|\mathbf{z}_k]\cdot \mathbb{E}[\mathbf{z}_q|\mathbf{z}_k]^\top
    \end{align}
    where $\mathbb{E}[\mathbf{z}_q|\mathbf{z}_k]$ is the predictive mean given in \eqref{eq: exp closed form} and $\mathbb{E}[\mathbf{z}_q\mathbf{z}_q^\top\mid \mathbf{z}_k]$ is given by the intergral, 
    \begin{equation} \label{eq:temp1}
        \begin{aligned}
            \mathbb{E}[\mathbf{z}_q\mathbf{z}_q^\top\mid \mathbf{z}_k] &= \int_{\mathbf{z}_q} \mathbf{z}_q\mathbf{z}_q^\top
     \Big(\int_{\mathbf{z}_0}p(\mathbf{z}_q\mathbf{z}_q^\top\mid \mathbf{z}_0)p(\mathbf{z}_0\mid\mathbf{z}_k)d\mathbf{z}_0\Big)d\mathbf{z}_q \\
            &= \int_{\mathbf{z}_0}\int_{\mathbf{z}_q} \mathbf{z}_q\mathbf{z}_q^\top p(\mathbf{z}_q\mathbf{z}_q^\top|\mathbf{z}_0)p(\mathbf{z}_0|\mathbf{z}_k)d\mathbf{z}_0d\mathbf{z}_q\\
            &=\int_{\mathbf{z}_0}\mathbb{E}[\mathbf{z}_q\mathbf{z}_q^\top|\mathbf{z}_0]p(\mathbf{z}_0|\mathbf{z}_k)d\mathbf{z}_0 = \mathbb{E}[\mathbb{E}[\mathbf{z}_q\mathbf{z}_q^\top\mid\mathbf{z}_0]\mid\mathbf{z}_k]
        \end{aligned}
    \end{equation}
    By the canonical representation of GP, we have 
    \begin{align*}
        \mathbf{z}_q\mid\mathbf{z}_0 &\sim \mathcal{N}(\mathcal{K}_{qo}(\mathcal{K}_0+\sigma I)^{-1}\mathbf{z}_0, \mathcal{K}_q-\mathcal{K}_{qo}(\mathcal{K}_0+\sigma I)^{-1}\mathcal{K}_{oq}).
    \end{align*}
    Thus, using the identity $\mathbb{E}(XX^\top) \ = \  \Sigma \ + \ mm^\top \text{ for } X \sim \mathcal{N}(m, \Sigma)$ we have,
    \begin{align*}
        \mathbb{E}[\mathbf{z}_q\mathbf{z}_q^\top\mid \mathbf{z}_0] 
        = \mathcal{K}_q-\mathcal{K}_{qo}(\mathcal{K}_0+\sigma I)^{-1}\mathcal{K}_{oq}  
        + \mathcal{K}_{qo}(\mathcal{K}_0+\sigma I)^{-1}\mathbf{z}_0\mathbf{z}_0^\top (\mathcal{K}_0+\sigma I)^{-\top} \mathcal{K}_{oq}
    \end{align*}
    Taking the expectation of $\mathbb{E}[\mathbf{z}_q\mathbf{z}_q^\top|\mathbf{z}_0]$ w.r.t $\mathbf{z}_0\mid \mathbf{z}_k$, gives
    \begin{align} \label{eq:temp2}
        \mathbb{E}_{\mathbf{z}_0|\mathbf{z}_k}[\mathbb{E}[\mathbf{z}_q\mathbf{z}_q^\top\mid \mathbf{z}_0]] &= \mathcal{K}_q-\mathcal{K}_{qo}(\mathcal{K}_0+\sigma I)^{-1}\mathcal{K}_{oq}  
        + \mathcal{K}_{qo}(\mathcal{K}_0+\sigma I)^{-1}\mathbb{E}[\mathbf{z}_0\mathbf{z}_0^\top\mid \mathbf{z}_k] (\mathcal{K}_0+\sigma I)^{-\top} \mathcal{K}_{oq}
    \end{align}
    Note that $\mathbf{z}_0|\mathbf{z}_k \sim \mathcal{N}(\mathcal{K}_{ok}(\mathcal{K}_k+\sigma I)^{-1}z_k, \mathcal{K}_0 - \mathcal{K}_{ok}(\mathcal{K}_k+\sigma I)^{-1}\mathcal{K}_{ko})$ due to the canonical GP representation, thus
    \begin{align} \label{eq:temp3}
        \mathbb{E}[\mathbf{z}_0\mathbf{z}_0^\top\mid \mathbf{z}_k] &= \mathcal{K}_0 - \mathcal{K}_{ok}(\mathcal{K}_k+\sigma I)^{-1}\mathcal{K}_{ok})
        +  \mathcal{K}_{ok}(\mathcal{K}_k+\sigma I)^{-1}\mathbf{z}_k \mathbf{z}_k^\top (\mathcal{K}_k+\sigma I)^{-\top} \mathcal{K}_{ko}
    \end{align}
    Finally, we can obtain the analytic form of the variance $\mathbb{V}[\mathbf{z}_q \mid \mathbf{z}_k]$ by combining equations \eqref{eq: variance formula}, \eqref{eq: exp closed form},
    \eqref{eq:temp1}, \eqref{eq:temp2}, \eqref{eq:temp3}.
}


\section{Additional Experiments}
    \subsection{Comparison with SGPA on CIFAR10-C}
    
    \subsection{Comparison with SGPA on CIFAR100-C}
    This section expands on our previous empirical comparison between SGPA and CGPT. Previously, we have shown that CGPT performs significantly better than SGPA in terms of both accuracy (MCC) and uncertainty calibration on the CIFAR10 dataset (see Table~\ref{tab:in-distribution} and Table~\ref{tab:OOD CIFAR}). Now, we will extend that comparison to a larger CIFAR100 dataset. In addition, to compare the robust performance of CGPT and SGPA on OOD learning scenarios, we also use the corrupted CIFAR100-C dataset. Similar to the CIFAR10-C dataset, the CIFAR100-C dataset also contains corrupted images from CIFAR100, which can be divided into $19$ types of distortion belonging to $4$ distortion categories: Noise, Blur, Weather and Digital. For each method, we calculate the mean performance metrics over the distortion types in each distortion category.

    
    %\par Besides CIFAR10, we also run additional image classification task on the larger CIFAR100 dataset. In this section, we compare both the in-distribution and OOD performances of CGPT and SGPA in terms of test accuracy and test calibration metrics: NLL, MCE and ECE. In order to compare the OOD robustness performances, we use the corrupted CIFAR100-C dataset. Much like the CIFAR10-C dataset, CIFAR100-C contains corrupted images from CIFAR100, which can be divided into 19 types of distortion belonging to 4 distortion categories: Noise, Blur, Weather and Digital. For each method, we choose the model with the best test accuracy on the clean test data on CIFAR100 for OOD evaluation, then we calculate the mean performance metrics over the distortion types in each distortion category. 
    
    \par All results are reported in Table \ref{tab:appx sgpa_cgpt_cifar100}, which shows that CGPT generally achieves better performance in terms of both (1) in-distribution accuracy and calibration on the authentic (no distortion) test data of CIFAR100 (see {\bf Original} column) and (2) out-of-distribution performance (accuracy and uncertainty calibration) on distorted test data derived from the CIFAR100-C dataset (see other columns). This is shown consistently across all distortion categories, resulting in a significantly improved averaged performance over all data distortion scenarios (see the {\bf Avg.} column).
        
        \begin{table*}[t!]
            \centering
            \caption{Accuracy and uncertainty calibration performance achieved by CGPT and SGPA on the original, in-distribution test data of CIFAR100 and distorted, out-of-distribution test data derived from CIFAR100-C. CGPT significantly outperforms SGPA in all cases.}
            \vspace{0.5em}
            \begin{tabularx}{\textwidth}{|X X X X X X X X|} 
                \toprule
                \textbf{Metric} & \textbf{Model} & \bf{Original} & \bf{Noise} & \bf{Blur} & \bf{Weather} & \bf{Digital} & \bf{Avg.}\\
                \midrule
                
                \multirow{2}{*}{Acc $\uparrow$} & SGPA & 46.94 & 25.04 & 32.62 & 33.20 & 33.38 & 31.32\\ 
                & CGPT & \textbf{49.60} & \textbf{27.83} & \textbf{34.83} & \textbf{35.15} & \textbf{34.68} & \textbf{33.29}\\
                \midrule
    
                 \multirow{2}{*}{NLL $\downarrow$} & SGPA & 2.16 & 4.00 & 3.31 & 3.21 & 3.34 & 3.45\\ 
                & CGPT & \textbf{2.05} & \textbf{3.87} & \textbf{3.10} & \textbf{3.09} & \textbf{3.25} & \textbf{3.32}\\
                \midrule
    
                 \multirow{2}{*}{MCE $\downarrow$} & SGPA & 0.25 & 0.44 & 0.39 & 0.37 & 0.37 & 0.39\\ 
                & CGPT & \textbf{0.24} & \textbf{0.43} & \textbf{0.35} & \textbf{0.36} & \textbf{0.36} & \textbf{0.37}\\
                \midrule
    
                 \multirow{2}{*}{ECE $\downarrow$} & SGPA & 0.15 & 0.26 & 0.24 & 0.22 & 0.22 & 0.23\\ 
                & CGPT & \textbf{0.12} & \textbf{0.25} & \textbf{0.19} & \textbf{0.20} & \textbf{0.20} & \textbf{0.21}\\
                \bottomrule
            \end{tabularx}
            \label{tab:appx sgpa_cgpt_cifar100}
        \end{table*}

    \subsection{ Comparison with non-GP Methods}
    % \begin{itemize}
    %     \item Symmetric Kernel attention on CoLA
    %     \item Asymmetric kernel attention on CoLA and CIFAR10
    % \end{itemize}
    This section expands on our previous comparison between CGPT and kernel attention (see Table~\ref{tab:cifar compare kernel}) which is also a kernel-based attention method. But, unlike CGPT and SGPA, it does not have uncertainty calibration. Previously, we have shown (in Table~\ref{tab:cifar compare kernel}) that CGPT achieves better performance than kernel attention with symmetric kernel. Now, we will expand that comparison towards kernel attention with asymmetric kernel as well. This is detailed below.
    
    %, which supports our point that allowing asymmetries in the attention matrix is essential. This however still raises the question of whether the proposed CGPT can achieve comparable or better performance than kernel attention with asymmetric kernel. This is now addressed in the below experiment, which further highlights the practical impact of our work.
    
    \par In particular, we train asymmetric kernel attention, dubbed {\bf Kernel (asym)} and compare with CGPT on an expanded set of benchmark datasets. Previously, we have only compared CGPT with {\bf Kernel (sym)} on the CIFAR10 dataset. Now, we will compare CGPT with {\bf Kernel (asym)} on CIFAR10, CIFAR100 (image classification) and CoLA (assessing linguistic acceptability) datasets. 
    
    As before, we report the in-distribution accuracy (MCC) as well as other uncertainty calibration metrics (NLL, MCE, ECE) achieved by the participating methods for each dataset in Table~\ref{tab:appx in-distribution}. In addition, we report their out-of-distribution performance on the CoLA dataset in the last row of Table \ref{tab:appx in-distribution}. For the CoLA experiments, we report the metric means and standard deviations over 9 independent runs while for the image datasets, we average the results over 3 independent runs.
    
    
    
    %will expand the performance of CGPT against variants of kernel attention, which are methods without uncertainty estimation. For kernel attention, we train two variants for evaluation, symmetric kernel attention, dubbed {\bf Kernel (sym)}, and asymmetric kernel attention, dubbed {\bf Kernel (asym)}. We evaluate the models' performance on three datasets, including CIFAR10 and CIFAR100 for image classification and CoLA for assessing linguistic acceptability. We report the in-distribution test accuracy/test MCC as well as the test calibration metrics (NLL, MCE, ECE) for all the datasets and we also report the out-of-distribution performances on the CoLA dataset in Table \ref{tab:appx in-distribution}. For the CoLA experiments, we report the metric means and standard deviations over 9 independent runs while for the image datasets, we average the results over 3 independent runs.

    \par The results in Table \ref{tab:appx in-distribution} show that in term of the uncertainty calibration metrics, CGPT expectedly outperforms {\bf Kernel (asym)} across all cases. In addition, in terms of accuracy/MCC, CGPT also outperforms {\bf Kernel (asym)} in most cases ($3$ out of $4$). Most notably, for the out-of-distribution (OOD) experiments on CoLA, we observe that CGPT achieves significantly better performance than asymmetric kernel attention across all metrics and tasks, which demonstrates conclusively the enhanced robustness of CGPT in OOD learning scenarios.
    
    
    %outperforms (on CIFAR10) or performs on par (on CoLA and CIFAR100) with kernel attention methods, however, CGPT achieves much better test calibration metrics than both of the kernel attention methods. For the out-of-distribution (OOD) experiments on CoLA, we observe that CGPT achieves the best performance in both OOD test MCC and calibration metrics, thus showing the robustness of CGPT in OOD tasks.

    \begin{table*}[t!]
        \centering
        \caption{Accuracy (MCC for CoLA) and calibration performance achieved by CGPT and asymmetric kernel attention evaluated on CIFAR10, CIFAR100 and CoLA datasets. The last row reports the performance of the above methods on an OOD scenario of the CoLA task. We report the mean and standard deviation over 3 independent runs for each experiment. CGPT outperforms asymmetric kernel attention on all calibration metrics while performing better or comparable (in most cases) in term of accuracy/MCC.}
        \vspace{0.5em}
        \begin{tabular}{ |l l c c c c| } 
            \toprule
            \textbf{Dataset} & \textbf{Model} & \bf{Accuracy/MCC $\uparrow$} & \bf{NLL $\downarrow$} & \bf{MCE $\downarrow$} & \bf{ECE $\downarrow$}\\
            \midrule
            
            % \multirow{2}{*}{CIFAR10} & Kernel (sym) & 76.12 $\pm$ 0.10 & 1.10 $\pm$ 0.02 & 0.61 $\pm$ 0.10 & 0.51 $\pm$ 0.06\\ 
             \multirow{2}{*}{CIFAR10} & Kernel (asym) & 74.88 $\pm$ 0.07 & 1.60 $\pm$ 0.02 & 0.42 $\pm$ 0.02 & 0.19 $\pm$ 0.01\\
            & CGPT (ours) & \textbf{76.21 $\pm$ 0.30} & \textbf{0.87 $\pm$ 0.03} & \textbf{0.27 $\pm$ 0.02} & \textbf{0.13 $\pm$ 0.05}\\
            \midrule
            

            % \multirow{3}{*}{CIFAR100} & Kernel  (sym) & \textbf{49.71 $\pm$ 0.55} & 3.65 $\pm$ 0.54 & 0.55 $\pm$ 0.01 & 0.37 $\pm$ 0.01\\ 
            \multirow{2}{*}{CIFAR100} & Kernel (asym) & 46.33 $\pm$ 0.29 & 3.63 $\pm$ 0.04 & 0.51 $\pm$ 0.01 & 0.35 $\pm$ 0.01\\
            & CGPT (ours) & \textbf{49.29} $\pm$ 0.31 & \textbf{2.11 $\pm$ 0.05} & \textbf{0.29 $\pm$ 0.03} & \textbf{0.16 $\pm$ 0.03}\\
            \midrule

            % \multirow{3}{*}{CoLA} & Kernel  (sym) & \textbf{26.14 $\pm$ 1.05} & 2.36 $\pm$ 0.25 & 0.54 $\pm$ 0.04 & 0.29 $\pm$ 0.01\\ 
            \multirow{2}{*}{CoLA} & Kernel (asym) & \textbf{25.25 $\pm$ 1.07} & 2.54 $\pm$ 0.10 & 0.57 $\pm$ 0.03 & 0.29 $\pm$ 0.01\\
            & CGPT (ours) & 22.69 $\pm$ 2.44 & \textbf{0.99 $\pm$ 0.07} & \textbf{0.46 $\pm$ 0.03} & \textbf{0.23 $\pm$ 0.01}\\
            \midrule

            % \multirow{3}{*}{CoLA (OOD)} & Kernel  (sym) & 17.97 $\pm$ 0.36 & 2.67 $\pm$ 0.01 & 0.56 $\pm$ 0.03 & 0.31 $\pm$ 0.01\\ 
            \multirow{2}{*}{CoLA (OOD)} & Kernel (asym) & 14.82 $\pm$ 1.46 & 3.00 $\pm$ 0.07 & 0.55 $\pm$ 0.04 & 0.31 $\pm$ 0.01\\
            & CGPT (ours) & \textbf{20.49 $\pm$ 1.83} & \textbf{1.02 $\pm$ 0.11} & \textbf{0.48 $\pm$ 0.05} & \textbf{0.24 $\pm$ 0.02}\\
            \bottomrule

            
            \end{tabular}
            \label{tab:appx in-distribution}
    \end{table*}

    
        

        \subsection{Correlated Gaussian Process Transformer (CGPT) Helps Reduce Oversmoothing in Transformers}
            \par Oversmoothing is a pathological behavior in transformer models that has recently been observed \cite{shi2022revisiting}. This behavior occurs when the representations learned in transformers converge to a low-rank sub-space as the number of attention blocks increases. This potential risk of degenerating representational capacity in transformers can be monitored or assessed by measuring the cosine similarities of the attention output of each block. As such, low values of the cosine similarity generally means high diversity among representations, which in turn suggests less risk of oversmoothing and vice versa. Thus, transformer methods with low cosine similarities of their attention outputs are more preferable.

            In this section, we will further show that CGPT interestingly has less risk regarding oversmoothing than the kernel attention variants. This is demonstrated via measuring and comparing the corresponding representational similarities between the output of their attention blocks, as described above.
            Specifically, we measure the similarities of the learned representations after the attention calculation and/or the feed-forward network (FFN) calculation after each attention block. 
            
            This is visually demonstrated in Fig.~\ref{fig:over_cifar10}, which shows that as the number of attention blocks increases, the cosine similarities between the representations learned with kernel attention methods become gradually higher. This implies that these representations will become more similar with each other as the models get deeper. On the contrary, the learned representations of CGPT have much lower cosine similarity as the model depth increases, which implies that CGPT will suffer less from oversmoothing than the kernel attention methods.
        
            \begin{figure}[t!]
                \centering
                \includegraphics[scale=0.58]{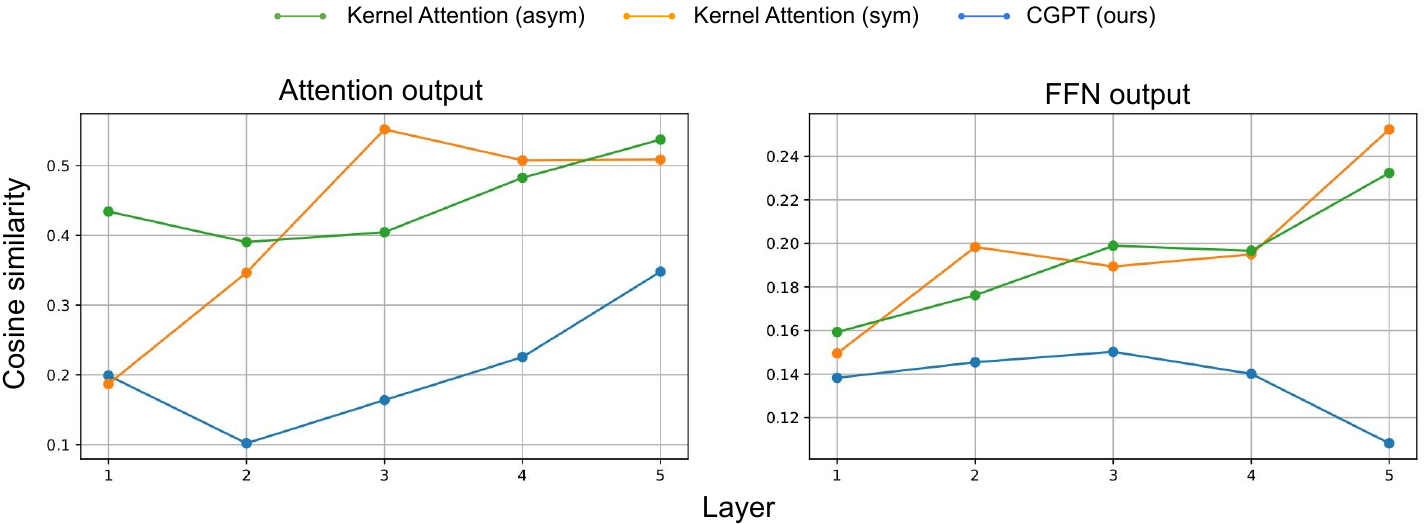}
                \vspace{-2em}
                \caption{The cosine similarity between the token representations after the attention calculation (left) and after the FFN layer (right)
                vs. the no. of attention layers of transformers models implementing the corresponding CGPT and kernel attention mechanisms on CIFAR10. Kernel attention methods appears more vulnerable to  oversmoothing as their attention representations become more similar as the number of attention layers increases. On the other hand, CGPT is much less vulnerable to oversmoothing as its learned representations are less similar and hence, more diverse.}
                \label{fig:over_cifar10_appex}
                \vspace{-0.2in}
            \end{figure}
            
            % \begin{figure}[]
            %     \centering
            %     \includegraphics[scale=0.6]{gptransformers/images/out_100.png}
            %     \caption{\textcolor{blue}{Long: For some reasons (probably some bugs), the FFN outputs of CGPT trained on CIFAR100 have higher cosine similarity than the kernel attention.}}
            %     \label{fig:over cifar100}
            % \end{figure}

        % \subsubsection{CGPT helps reduce head-redundancy in transformers}

    \subsection{Out-of-Distribution Detection}
        \par This section evaluates and compares the performance of CGPT and SGPA on OOD detection task for image classification. In this task, our goal is to determine if a test data point originates from the same distribution as the training data or from a different distribution \cite{hendrycks2016baseline}, \cite{yang2022openood}. 
        For both methods, we use the CIFAR10 dataset as the in-distribution dataset for OOD detection. 
        
        We choose $4$ different common image datasets for the OOD detection task which includes Textures, LSUNCrop, LSUNResize and TinyImageNetCrop as our OOD datasets. In addition, we also need a detector to distinguish if the data point is from a different distribution. For this, we choose $4$ state-of-the-art detectors to be used in our experiments: KLMatching \cite{hendrycks2019scaling}, Maximum Softmax Probability (MaxSoftmax) \cite{hendrycks2016baseline}, Entropy Maximization (Entropy) \cite{chan2021entropy} and Energy-Based OOD Detection (EnergyBased) \cite{liu2020energy}. We use the following standard OOD detection metrics for evaluation, which includes (1) the area under the Receiver Operating Characteristic curve (AUROC), (2) the in-distribution and out-distribution area under the Precision-Recall curve (AUPR-IN and AUPR-OUT) and (3) the false positive rate when the true positive rate is equal to 95\% (FPR@95). 

        \par For each method, we evaluate the OOD performance of CGPT and SGPA measured using the above metrics on the 4 OOD datasets and report the mean metrics for each of the 4 detectors. All results are reported in Table \ref{tab:ood detection} which shows that CGPT again outperforms SGPA in terms of OOD performance with respect to all the detectors and most of the metrics. Concretely, CGPT achieves better average AUROC, AUPR-IN and AUPR-OUT than SGPA, and performs comparably with SGPA on FPR@95.
        
        \begin{table*}[t!]
            \centering
            \caption{Averaged OOD detection performance achieved by CGPT and SGPA over $4$ datasets (Textures, LSUNCrop, LSUNResize and TinyImageNetCrop). For each method, the average OOD performance is reported for each detector. CGPT outperforms SGPA in most OOD detection metrics, suggesting its strong advantage over SGPA on OOD detection task.}
            \vspace{0.5em}
            \small
            \begin{tabularx}{\textwidth}{|X X X X X X|} 
                \toprule
                \textbf{Model} & \textbf{Detector} & \bf{AUROC $\uparrow$} & \bf{AUPR-IN $\uparrow$} & \bf{AUPR-OUT $\uparrow$} & \bf{FPR@95 $\uparrow$}\\
                \midrule
                
                \multirow{5}{*}{CGPT} & KLMatching & 63.25 & \textbf{60.27} & 61.62 & \textbf{93.18}\\
                
                & MaxSoftmax & \textbf{68.10} & \textbf{60.85} & \textbf{73.53} & 74.51\\
                
                & Entropy & \textbf{69.97} & \textbf{63.34} & \textbf{74.65} & 73.80\\
                
                & Energy-Based & \textbf{73.13} & \textbf{63.01} & \textbf{78.58} & 66.91\\
                
                & Average & \textbf{69.58} & \textbf{69.25} & \textbf{70.44} & 70.41\\
                \midrule

                \multirow{5}{*}{SGPA} & KLMatching & \textbf{63.66} & 59.88 & 63.94 & 88.62\\
                
                & MaxSoftmax & 66.78 & 59.18 & 72.55 & \textbf{75.71}\\
                
                & Entropy & 68.12 & 61.20 & 73.18 & \textbf{75.80}\\
                
                & Energy-Based & 72.55 & 62.95 & 78.14 & \textbf{68.27}\\
                
                & Average & 69.03 & 68.56 & 69.58 & \textbf{70.48}\\
    
                 
                \bottomrule
            \end{tabularx}
            \vspace{-0.2in}
            \label{tab:ood detection}
        \end{table*}

    



\section{Further Experiment Details}
    \par \textbf{General Settings.} We adopted the same experiments settings from ~\cite{chen2023calibrating} in our own empirical studies. For SGPA and kernel attention methods, we use the ARD-RBF kernel \cite{Rasmussen06}
    $ \kappa(\mathbf{x}, \mathbf{x}') = \sigma_s^2 \exp({-0.5\sum_{i=1}^d (x_i-x'_i)^2/\sigma_i^2})$ for image classification, and an exponential of scaled dot product variant $\kappa(\mathbf{x},\mathbf{x}')=\sigma_s^2 \exp(\sum_{i=1}^d x_ix'_i/\sigma_i^2)$ for the linguistic acceptability task. Here, $\mathbf{x}$ 
    and $\mathbf{x}'$ are $d$-dimensional inputs while $\sigma_s^2$ denotes the output variance and $\{\sigma_i^2\}_{i=1}^d$ are the length scales. 
    
    For CGPT, we use the parameter-free squared exponential kernel function $\kappa_o(\mathbf{x}, \mathbf{x}') = \mathrm{exp}(-0.5 \|\mathbf{x} - \mathbf{x}'\|^2)$ and compute the necessary kernels using $\kappa_o(\mathbf{x}, \mathbf{x}')$ in Eqn. \eqref{eq: kernel q k} and \eqref{eq: cross-kernel func}. We set the parameters $\sigma_k$ and $\sigma_q$ in \eqref{eq: kernel q k}, \eqref{eq: cross-kernel func} to be learnable parameters. All models are trained from scratch with random initialization using the standard Adam optimizer. All of our experiments are conducted on two NVIDIA GeForce RTX 3090 GPUs with 24Gb in memory each. 

    \par \textbf{Image Classification.} For the CIFAR10 dataset, we use Vision Transformers (ViT) \cite{dosovitskiy2020image} with 5 MHSA layers, each layer has 4 attention heads. We set the hidden dimension to be 128. For the CIFAR100 dataset, we also use ViT, with 6 MHSA layers with 4 attention heads in each layer and the hidden dimension set to be 256. The images in both of the datasets are of size 32x32 and are tokenized using 4x4 patches, resulting in a sequence of length 64. 
    
    The number of inducing points in SGPA \cite{chen2023calibrating} are set to be 32. For both datasets, the initial learning rate is 5e-4, we set the batch size to 100 and train the models for 600 epochs. For evaluation, we choose the model with the best validation accuracy computed after each 50 epochs. For the OOD tasks on CIFAR10-C and CIFAR100-C, we use the models trained on the clean data and use the corrputed datasets to evaluate the OOD performances.

    \par \textbf{Linguistic Acceptability.} For the CoLA dataset, we use a standard transformer with 2 MHSA layers with 4 attention heads in each layer. We set the hidden dimension and the embedding dimension to be 256 and 128 respectively. The batch size is chosen to be 32. We choose the number of inducing points for SGPA to be 5. All the models are trained with initial learning rate 5e-4 for 50 epochs. The model at the final epoch is used for evaluation. The original CoLA dataset consists of 516 OOD samples, which are used to evaluate the OOD performance of the models.


% \subsection{More tasks}
%         \begin{enumerate}
%         \item OOD detection (Done)
%         \item Compare with kernel attention (Done)
%         \item ViT on CIFAR100 (Done) and CIFAR100-C (done)
%         \item Oversmoothing for attention output (Done - weird behavior in fig \ref{fig:over cifar100})
%         \item head redundancy analysis for (CGPT, SGPA, Kernel, softmax) (cosine similarity too small)
%         \item Sym CGPT vs asym CGPT (nan encountered)
%         % \item small scale data (SGPA)
            
            
%         \end{enumerate}
